# Supplementary material for: Birth, life, and death of a dipolar supersolid
Source: arXiv:2101.06975 ancillary file (2021-03-22)
Supplement: Supplementary file 1 [file Evaporation_Supmat_PRL.pdf]

# Supplementary Material: Birth, life, and death of a dipolar supersolid

Maximilian Sohmen,[1,2] Claudia Politi,[1,2] Lauritz Klaus,[1,2] Lauriane Chomaz,[2]
Manfred J. Mark,[1,2] Matthew A. Norcia,[1] and Francesca Ferlaino[1,2,*]

[1] *Institut für Quantenoptik und Quanteninformation, Österreichische Akademie der Wissenschaften, Innsbruck, Austria*

[2] *Institut für Experimentalphysik, Universität Innsbruck, Austria*

(Dated: March 12, 2021)

## CALCULATION OF DENSITY-DENSITY CORRELATOR

We define our correlator as

$$C(d) = \langle \int n(x)\, n(x+d)\, \mathrm{d}x \rangle\,, \tag{1}$$

where $n(x)$ is the projected density at position $x$ along our cigar-shaped trap, and the expectation value $\langle \ldots \rangle$ is calculated over different runs of the experiment. In practice, we follow a standard procedure (e. g., Ref. [1]) and calculate the correlator by computing the square of the Fourier transform of each image to obtain its power spectral density, then Fourier transform again to obtain its autocorrelation function. The autocorrelation functions for the different images in the sample are then averaged to obtain $C(d)$. Note that we do not normalize this as is typical for a noise correlator, as we are interested in the structure of the density profile and not specifically in its fluctuations. To extract the correlation length, we first subtract off a slowly varying background that represents the envelope of our density profile from $C(d)$ to obtain $C'(d)$, shown in Fig. 2b of the main text. We then fit the product of a Gaussian and a cosine with spatial frequency $k_m = 2\pi/x_m$ corresponding to the in-trap modulation wavelength $x_m$, i. e. $\cos(k_m x)\exp(-x^2/2L^2)$, and define the correlation length as $L$.

## CALCULATION OF COHERENCE QUANTITIES

As described in the main text, we evaluate the coherence of our droplet array by imaging the sample after TOF expansion and Fourier transformation ($\mathcal{F}$) of the projected density profile $n(x')$ (cf. Fig. 1c in main text), where in-situ distances $x$ and the corresponding transforms are denoted as $x \xrightarrow{\mathrm{TOF}} x' \xrightarrow{\mathcal{F}} x''$ [2]. For each experimental repetition $i$ this yields a phasor

$$\tilde{P}_i(x'') = \mathcal{F}\{n(x')\}_{x''}. \tag{2}$$

We can calculate the incoherent and coherent means of the Fourier amplitudes over the experimental repetitions $i$, writing

$$\tilde{A}_M(x'') = \langle |\tilde{P}_i(x'')| \rangle_i \quad \text{and} \quad \tilde{A}_\Phi(x'') = |\langle \tilde{P}_i(x'') \rangle_i|, \tag{3}$$

respectively.

The quantities $A_M$ and $A_\Phi$ from the main text are closely connected to $\tilde{A}_M(x'')$ and $\tilde{A}_\Phi(x'')$. To disentangle the spectral amplitude from the coherent atom number (i. e., the area under the density profile), we calculate the rescaled phasors

$$P_i(x'') = \frac{\tilde{P}_i(x'')}{\int |\tilde{P}_i(x'')| \mathrm{d}x''} \tag{4}$$

mentioned in the main text. The amplitude means corresponding to the in-trap modulation at wavelength $x_m$ are then given by

$$A_M = \langle |P_i(x''_m)| \rangle_i \quad \text{and} \quad A_\Phi = |\langle P_i(x''_m) \rangle_i|. \tag{5}$$

## SUPPLEMENTARY DATA FOR FIG. 2

The data of Fig. 2 of the main text is obtained from in-situ images of samples created via the 'fast ramp' evaporation procedure. From corresponding TOF images, taken after the data of Fig. 2, we can study the time evolution of $\tilde{A}_M(x'')$ and $\tilde{A}_\Phi(x'')$ over the hold time $t_h$. After about a hundred milliseconds a sidepeak has developped in $\tilde{A}_M(x'')$, corresponding to the in-trap density modulation at $x_m \sim 3.5\,\mu\mathrm{m}$ wavelength. A corresponding peak develops in $\tilde{A}_\Phi(x'')$, signalling growing coherence between the droplets. In Fig. S1 we plot a direct comparison of the rescaled Fourier amplitude means, $A_M$ and $A_\Phi$, calculated at $x''_m = 3.5\,\mu\mathrm{m}$. We see that both $A_M$ and $A_\Phi$ increase with $t_h$ and the increase of modulation strength starts before the development of phase coherence.

For reference, we plot in Fig. S2 the evolution of the total ($N$) and coherent ($N_c$) atom number for the data set of Fig. 2 of the main text, obtained using the 'fast ramp' evaporation protocol.

## SUPPLEMENTARY DATA FOR FIG. 4

Fig. 4 of the main text shows the death of the supersolid over long hold times $t_h$. Here we compare in Fig. S3 the evolution of $A_M$ and $A_\Phi$, calculated at the sidepeak

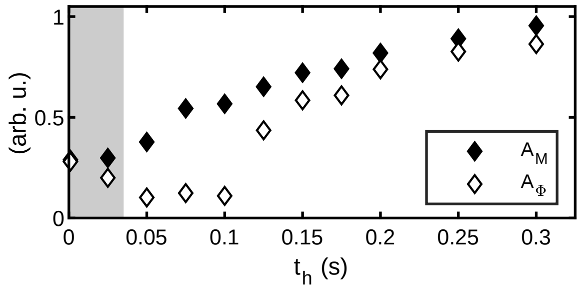


FIG. S1. **Development of coherence after the 'fast ramp' evaporation.** Evolution of the means $A_M$ and $A_\Phi$ from the TOF profiles during the hold time $t_h$. The gray shading marks the region where due to low overall signal the rescaling of the phasors (Eq. 4) is dominated by noise.

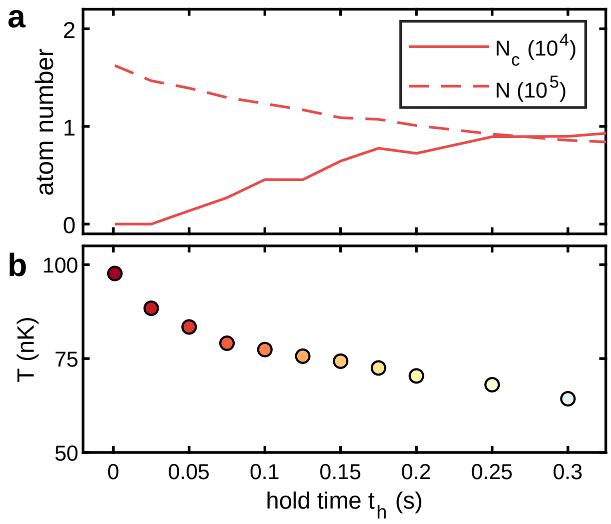


FIG. S2. **Atom number and temperature after the 'fast ramp' evaporation. a.** Evolution of total ($N$, dashed) and condensed atom number ($N_c$, solid line). **b.** Evolution of the temperature, as extracted by a Bose-enhanced Gaussian fit to the background cloud of thermal atoms [3].

in $\tilde{A}_M$ at $x'' = 3.5\,\mu\text{m}$, during the death of the supersolid. We start our discussion looking at $A_M$, the measure for in-trap modulation. $A_M$ stays roughly constant for around 600 ms before it starts to decay. At above $\sim 1.1\,\text{s}$ (gray shading in Fig. S3), the sidepeak in $\tilde{A}_M$ around $x'' = 3.5\,\mu\text{m}$ has vanished. However, $A_M$ does not go straight to zero, since when the modulation disappears, the fundamental peak (around $x'' = 0$) broadens to $x'' > 3.5\,\mu\text{m}$ because the condensate size becomes comparable to the (former) droplet spacing. From this point onwards, $A_M$ cannot be used anymore as a measure for modulation. Recall that in the in-situ analysis (Fig. 4 of the main text) a very similar behaviour was observed, with maximal modulation until $\sim 600\,\text{ms}$ and modulation having disappeared by $\sim 1.1\,\text{s}$.

Now turning to $A_\Phi$, we note that over the full duration of this process $A_M$ and $A_\Phi$ (which is bounded by $A_M$) evolve closely together, suggesting that coherence is maintained in the sample throughout the life and death.

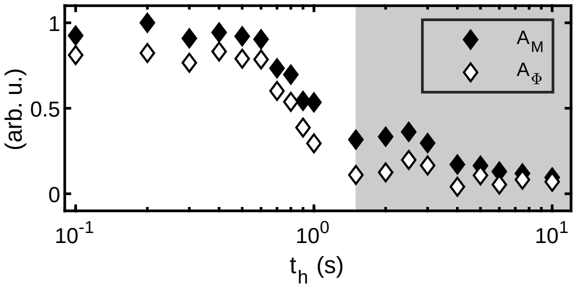


FIG. S3. **Coherence properties during the death of the supersolid.** Evolution of the means $A_M$ and $A_\Phi$ from the TOF profiles during $t_h$ after a 'slow ramp' evaporation. The gray shading marks the region from when on the sidepeaks in $\tilde{A}_M$ corresponding to in-trap modulation have disappeared and $A_M$ is not a good measure for modulation anymore.

## EVAPORATION RAMPS

In the experiment, once the atoms are loaded into our crossed optical dipole trap (ODT), we perform a near-exponential evaporation ramp of trap power, approximated by piecewise linear ramp sections. The trap frequencies after the penultimate ramp are around $\omega'_{x,y,z} = 2\pi\times(39, 178, 174)\,\text{s}^{-1}$, where we typically have around $N = 3\times10^5$ atoms at around 200 nK. From here, we ramp the power of the ODT linearly down to the final value, giving around $\omega_{x,y,z} = 2\pi\times(36, 88, 141)\,\text{s}^{-1}$. This procedure yields the atom numbers and temperatures presented in Figs. 3–4 of the main text and Fig. S2.

## IMAGING SPECIFICATIONS

The images shown in this work have been recorded using a new imaging system recently installed in our experiment. The direction of view of the new system is vertical (counter-directed to gravity).

Images from our imaging along the horizontal direction (as in our earlier works, see, e. g., Refs [4, 5]), in contrast, suffer from the fact that the line of sight is at 45° with respect to the axis connecting the droplets, leading to a small apparent fringe spacing and to the interference peaks partially hiding each other; additionally the interference peaks do not lie in a single focus plane. These drawbacks were eliminated with the vertical imaging setup, which is why the images are much clearer to interpret now.

The fundamental resolution of this imaging system, applicable to in-trap images and characterised by the

Rayleigh criterion, has been measured offline to be approximately 700 nm. We report micron-scale resolution as a conservative claim that accounts for possible alignment imperfections in the finally installed condition, and a reduction of the imaging aperture to increase depth of field. The pixel size of our camera is smaller than the imaging resolution, corresponding to approximately 400 nm at the location of the atoms. Additionally, the images displayed have been supersampled to allow them to be rotated while maintaining resolution.

---

* Correspondence should be addressed to Francesca.Ferlaino@uibk.ac.at

[1] S. Fölling, F. Gerbier, A. Widera, O. Mandel, T. Gericke, and I. Bloch, Spatial quantum noise interferometry in expanding ultracold atom clouds, Nature **434**, 481 (2005).

[2] We avoid identifying the positions of atoms after TOF with the in-trap momenta (i. e. $k \equiv x'$) because we know from simulation and experiment that in the first few milliseconds of TOF the droplets can still be loosely bound and the expansion is not purely ballistic.

[3] W. Ketterle, D. S. Durfee, and D. M. Stamper-Kurn, Making, probing and understanding Bose–Einstein condensates, Proceedings of the International School of Physics "Enrico Fermi" (1999).

[4] L. Chomaz, R. M. W. van Bijnen, D. Petter, G. Faraoni, S. Baier, J.-H. Becher, M. J. Mark, F. Wächtler, L. Santos, and F. Ferlaino, Observation of roton mode population in a dipolar quantum gas, Nat. Phys. **14**, 442 (2018).

[5] P. Ilzhöfer, M. Sohmen, G. Durastante, C. Politi, A. Trautmann, G. Natale, G. Morpurgo, T. Giamarchi, L. Chomaz, M. J. Mark, and F. Ferlaino, Phase coherence in out-of-equilibrium supersolid states of ultracold dipolar atoms, Nature Physics 10.1038/s41567-020-01100-3 (2021).
